# Supplementary material for: HOIGaze: Gaze Estimation During Hand-Object Interactions in Extended Reality Exploiting Eye-Hand-Head Coordination
Source: arXiv:2504.19828 source file (2025-04-28)
Supplement: Supplementary file 1 [file supp.tex]

%\section{Experiments and Results}

\section{Attended Hand Recognition Accuracy and Gaze Estimation Performance}
Our attended hand recogniser achieves an accuracy of $83.0\%$ on HOT3D (Cross-User), $83.6\%$ on HOT3D (Cross-Scene), and $86.5\%$ on ADT, respectively.
To better understand the error distribution of our method, we further calculated the mean angular errors of different methods when the recognised attended hand is correct or wrong.
We can see from \autoref{tab:attended_hand} that our method significantly outperforms other methods when the recognised attended hand is correct, achieving an improvement of $17.5\%$ ($9.03^\circ$ \textit{vs.} $10.94^\circ$) on HOT3D (Cross-User), $14.3\%$ ($8.27^\circ$ \textit{vs.} $9.65^\circ$) on HOT3D (Cross-Scene), and $8.1\%$ ($8.52^\circ$ \textit{vs.} $9.27^\circ$) on ADT.
We also find that when the recognised attended hand is wrong, our method can achieve superior or comparable performance with the state of the art, demonstrating the robustness of our method.

\begin{table}[t] 
	\centering
	% set the caption of the table.
	\caption{Attended hand recognition accuracies and mean angular errors of different methods on the HOT3D and ADT datasets when the recognised attended hand is correct (\checkmark) or wrong ($\times$). Best results are in bold.} \label{tab:attended_hand} 
        \resizebox{0.5\textwidth}{!}{
	\begin{tabular}{cccc}
		\toprule
		      & \textbf{HOT3D-User} & \textbf{HOT3D-Scene} & \textbf{ADT} \\ \hline    
    Recognition Accuracy & 83.0\% & 83.6\% & 86.5\%\\
    \midrule
    \textit{Head Direction} \checkmark & $22.96^\circ$ & $23.11^\circ$ & $22.25^\circ$\\
    \textit{DGaze} \checkmark & $14.27^\circ$ & $12.79^\circ$ & $9.88^\circ$\\
    \textit{FixationNet} \checkmark & $13.95^\circ$ & $12.52^\circ$ & $9.91^\circ$\\
    \textit{Pose2Gaze} \checkmark & $10.94^\circ$ & $9.65^\circ$ & $9.27^\circ$\\
    Ours \checkmark & $\textbf{9.03}^\circ$ & $\textbf{8.27}^\circ$ & $\textbf{8.52}^\circ$\\
    \midrule
    \textit{Head Direction} $\times$ & $24.38^\circ$ & $23.66^\circ$ & $22.28^\circ$\\
    \textit{DGaze} $\times$ & $14.40^\circ$ & $12.87^\circ$ & $10.21^\circ$\\
    \textit{FixationNet} $\times$ & $14.25^\circ$ & $12.55^\circ$ & $9.99^\circ$\\
    \textit{Pose2Gaze} $\times$ & $11.89^\circ$ & $10.54^\circ$ & $\textbf{9.80}^\circ$\\
    Ours $\times$ & $\textbf{11.01}^\circ$ & $\textbf{10.53}^\circ$ & $10.47^\circ$\\
    \bottomrule
	\end{tabular}}
\end{table}

\section{Ablation Study}
\begin{table}[tbp] 
	\centering
	% set the caption of the table.
	\caption{Mean angular errors of our method's different ablated versions on the HOT3D and ADT datasets. Best results are in bold.} \label{tab:ablation} 
        \resizebox{0.5\textwidth}{!}{
	\begin{tabular}{cccc}
		\toprule
		      & \textbf{HOT3D-User} & \textbf{HOT3D-Scene} & \textbf{ADT} \\ \hline
    w/o self-attention & $9.80^\circ$ & $8.68^\circ$ & $9.08^\circ$\\
    w/o cross-attention & $10.22^\circ$ & $8.98^\circ$ & $8.99^\circ$\\                                 
    Ours & $\textbf{9.37}^\circ$ & $\textbf{8.64}^\circ$ & $\textbf{8.78}^\circ$\\
    \midrule
    recogniser GCN 0 & $9.75^\circ$ & $8.78^\circ$ & $8.99^\circ$\\
    recogniser GCN 1 & $9.56^\circ$ & $8.74^\circ$ & $8.89^\circ$\\
    recogniser GCN 2 (Ours) & $\textbf{9.37}^\circ$ & $\textbf{8.64}^\circ$ & $\textbf{8.78}^\circ$\\
    recogniser GCN 4 & $9.60^\circ$ & $8.86^\circ$ & $8.96^\circ$\\
    recogniser GCN 8 & $9.69^\circ$ & $8.71^\circ$ & $8.96^\circ$\\
    \midrule    
    estimator GCN 0 & $9.87^\circ$ & $9.13^\circ$ & $9.20^\circ$\\
    estimator GCN 1 & $10.24^\circ$ & $9.01^\circ$ & $9.11^\circ$\\
    estimator GCN 2 & $9.85^\circ$ & $8.66^\circ$ & $\textbf{8.74}^\circ$\\
    estimator GCN 4 (Ours) & $\textbf{9.37}^\circ$ & $\textbf{8.64}^\circ$ & $8.78^\circ$\\
    estimator GCN 8 & $9.69^\circ$ & $8.65^\circ$ & $8.84^\circ$\\
    \midrule
    scene object 0 & $10.34^\circ$ & $9.19^\circ$ & $9.03^\circ$ \\ %\hline                
    scene object 1 (Ours) & $\textbf{9.37}^\circ$ & $8.64^\circ$ & $\textbf{8.78}^\circ$\\
    scene object 2 & $9.59^\circ$ & $\textbf{8.61}^\circ$ & $8.91^\circ$\\
    scene object 3 & $9.88^\circ$ & $8.72^\circ$ & $9.36^\circ$\\
    scene object 4 & $9.79^\circ$ & $8.68^\circ$ & $9.16^\circ$\\
    \bottomrule
	\end{tabular}}
\end{table}

\paragraph{Cross-Modal Transformer}
We removed the self-attention and cross-attention used in the cross-modal Transformers respectively to re-train our method.
The results in \autoref{tab:ablation} show that our method achieves significantly better performances than the ablated versions (paired Wilcoxon signed-rank test, $p<0.01$), demonstrating that both the self-attention and cross-attention help improve our method's performance.

\paragraph{GCN in Attended Hand Recogniser and Gaze Estimator}
We changed the number of residual GCN layers used in our attended hand recogniser and gaze estimator respectively to re-train our method.
We can see from the results in \autoref{tab:ablation} that using two residual GCNs in the attended hand recogniser and four residual GCNs in the gaze estimator achieves the best performance.
One exception is that using two residual GCNs in the gaze estimator achieves better performance than using four residual GCNs on the ADT dataset ($8.74^\circ$ \textit{vs.} $8.78^\circ$).
This is because we trained our method on ADT using a static hand gesture that requires fewer GCN layers to process.

\paragraph{Scene Object Number}
We changed the number of scene objects to re-train our method.
As can be seen from the results in \autoref{tab:ablation} that using the nearest scene object achieves the best performance.
One exception is that using the nearest two objects achieves better performance than using one object on the HOT3D dataset for cross-scene evaluation ($8.61^\circ$ \textit{vs.} $8.64^\circ$).
This is because different environments usually have different scene layouts and thus our method needs more scene object information to improve its generalisation ability for different environments.
